# Supplementary material for: Profit Shifting of Multinational Corporations Worldwide
Source: arXiv:2201.08444 source file (2023-12-05)
Supplement: Supplementary file 1 [file appendix_variables.pdf]

| Variable           | Description                                | Source |
|--------------------|--------------------------------------------|--------|
| iso3               | ISO-3 code                                 | N/A    |
| revt, emp, pi, txc | Revenue, employees, profits and cash taxes | CBCR   |

### Bilateral Variables

|                        |                                                                         |                |
|------------------------|-------------------------------------------------------------------------|----------------|
| ln_Import              | Log of total imports from origin to destination                         | COMTRADE       |
| ln_Export              | Log of total exports from origin to destination                         | COMTRADE       |
| ln_FDI_inward          | Log of total FDI from orogin to destination                             | IMF CDIS       |
| ln_FDDI_outward        | Log of total FDI from destination to origin                             | IMF CDIS       |
| ln_PortI_inward        | Log of total portfolio investment from orogin to destination            | IMF CPIS       |
| ln_PortI_outward       | Log of total portfolio investment from destination to origin            | IMF CPIS       |
| ln_dClaims             | Log of total banking claims (derived from partners)                     | BIS Table A6.2 |
| ln_dLiabilities        | Log of total banking liabilities (derived from partners)                | BIS Table A6.2 |
| ln_distw               | Ln of distance between countries                                        | CEPII GravData |
| tdiff                  | Time zones difference (hours)                                           | CEPII GravData |
| transition_legalchange | Dummy, 1 if common legal origin changed since transition                | CEPII GravData |
| eu_to_acp              | Dummy, EU/member exporting to an ACP country (a preferent               | CEPII GravData |
| acp_to_eu              | Dummy, ACP country exporting to an EU/member (a preferent               | CEPII GravData |
| col45                  | Dummy, colonial relationship post 1945                                  | CEPII GravData |
| col_fr                 | Dummy, origin of colonial relationship post 1945                        | CEPII GravData |
| col_to                 | Dummy, destination of colonial relationship post 1945                   | CEPII GravData |
| colony                 | Dummy, colonial relationship (ever)                                     | CEPII GravData |
| comcol                 | Dummy, common colonizer post 1945                                       | CEPII GravData |
| comcur                 | Dummy, common currency                                                  | CEPII GravData |
| comlang_ethno          | Dummy, common language (>9% population)                                 | CEPII GravData |
| comlang_off            | Dummy, common official language                                         | CEPII GravData |
| comleg_posttrans       | Dummy, common legal origins after transition                            | CEPII GravData |
| comleg_pretrans        | Dummy, common legal origins before transition                           | CEPII GravData |
| comrelig               | Religious proximity index                                               | CEPII GravData |
| contig                 | Dummy, contiguity                                                       | CEPII GravData |
| curcol                 | Dummy, current colonial relationship                                    | CEPII GravData |
| cursib                 | Dummy, current sibling relationship (common colonizer)                  | CEPII GravData |
| sibling                | Dummy, ever sibling relationship (common colonizer)                     | CEPII GravData |
| fta_wto                | Dummy, regional trade agreement (WTO)                                   | CEPII GravData |
| gsp                    | Dummy if donator in Generalized System of Preferences                   | CEPII GravData |
| heg_o                  | Dummy, 1 if origin is current of former hegemon of destination          | CEPII GravData |
| heg_d                  | Dummy, 1 if destination is current of former hegemon of origin          | CEPII GravData |
| gsp_d_d                | Dummy, 1 if origin is donator in Generalized System of Preferences      | CEPII GravData |
| gsp_o_d                | Dummy, 1 if destination is donator in Generalized System of Preferences | CEPII GravData |

### Unilateral Variables: Included for the reporting and partner countries

|                                     |                                                                                  |                |
|-------------------------------------|----------------------------------------------------------------------------------|----------------|
| Legislative/historical/Geographical |                                                                                  |                |
| entry_proc                          | Start-up procedures to register a business (Number)                              | CEPII GravData |
| entry_time                          | Time required to start a business (days)                                         | CEPII GravData |
| entry_tp                            | Days+Procedures to start a business                                              | CEPII GravData |
| gatt                                | GATT member                                                                      | CEPII GravData |
| EU28                                | Dummy, country belonging to the EU-28                                            | N/A            |
| OECD                                | Dummy, country belonging to the OECD                                             | N/A            |
| Ukt                                 | Dummy, UK-territory                                                              | N/A            |
| region_tjn                          | Region                                                                           | TJN            |
| ln_area                             | Log of area in sq. kms                                                           | CEPII GravData |
| ln_entry_cost                       | Log of cost of business start-up procedures (log of % GNI per capita)            | CEPII GravData |
| english                             | Official language 1 in the CEPII GeoDist dataset                                 | CEPII GeoDist  |
| governance                          | First PCA component of the six dimensions of the Worldwide Governance Indicators | WBD            |

#### Socio-economic and financial

|                     |                                 |                                                                 |
|---------------------|---------------------------------|-----------------------------------------------------------------|
| Nurses_per_1000     | Nurses per 1000 inhabitants     | WBD                                                             |
| Physicians_per_1000 | Doctors per 1000 inhabitants    | WBD                                                             |
| ln_Nurses           | Log of number of nurses         |                                                                 |
| ln_physician        | Log of number of doctors        |                                                                 |
| ln_pop              | Population (source CEPII)       | CEPII GravData                                                  |
| ln_population       | Population (source WBD)         | WBD                                                             |
| ln_POP_int          | Population (manually completed) | Following order of preference: WBD, UN, CIA, manually completed |
| ln_GDP_int          | GDP (manually completed)        | Following order of preference: WBD, UN, CIA, manually completed |
| ln_gdp_d            | GDP                             | CEPII GravData                                                  |

|                               |                                                                                            |                                            |
|-------------------------------|--------------------------------------------------------------------------------------------|--------------------------------------------|
| ln_gdpcap_d                   | GDP per capita                                                                             | CEPII GravData                             |
| ln_gdppc_d                    | GDP per capita                                                                             | ln_GDP_int - ln_POP_int                    |
| ln_Health_expenditure_gdp     | Log of health expenditure (% of gdp)                                                       | WBD                                        |
| ln_uhnwi                      | Log10 of the number of high net worth individuals (adults with net worth > 1M USD)         | Global Wealth Report 2018 by Credit Suisse |
| ratings                       | Trading Economic credit rating, composed from the credit ratings of Moody's, S&P and Fitch | Feb. 2019 tradingeconomics.com             |
| ln_n_companies_orb            | Log of number of MNCs with a turnover higher than 750M in O Orbis                          |                                            |
| ln_GreenfieldFDI_inward       | Total greenfield FDI into the country                                                      | UNCTAD                                     |
| ln_GreenfieldFDI_outward      | Total greenfield FDI out of the country                                                    | UNCTAD                                     |
| ln_BIS                        | Log of total consolidated banking claims on an immediate country                           | BIS (Table B4)                             |
| ln_ExternalDebtStocks         | Log of External Debt Stock                                                                 | WBD                                        |
| ln_consumption                | Log10 of final consumption expenditure by households and non-profit institutions           | Mean 2014-2018NE.CON.PRVT.KD               |
| ln_gfcf                       | Log10 of gross fixed capital formation (constant 2010 USD)                                 | Mean 2014-2018NE.GDI.FTOT.KD               |
| ln_FDI_Inflows_WDI_d          | Log of total FDI inflows                                                                   | WBD                                        |
| ln_imports_wbd                | Log of total imports in the country                                                        | WBD                                        |
| ln_ip_payments_wbd            | Log of IP payments in the country                                                          | WBD                                        |
| ln_ip_receipts_wbd            | Log of IP receipts in the country                                                          | WBD                                        |
| ln_exports_wbd                | Log of total exports in the country                                                        | WBD                                        |
| ln_month_wage                 | Log of monthly wage                                                                        | ILO                                        |
| ln_govt_exp_educ_sgdp_wb      | Log of government expenditure in education (%GDP)                                          | WBD                                        |
| ln_who_gvt_health_expenditure | Log of public expenditure in health care                                                   | WHO                                        |
| ln_cit_revenue                | Log of government revenue from corporate income tax                                        | UNU - WIDER GRD                            |
| ln_resource_revenue           | Log of government revenue from resource taxes and fees                                     | UNU - WIDER GRD                            |
| ln_resource_taxes             | Log of government revenue from resource taxes                                              | UNU - WIDER GRD                            |
| ln_resource_revenue_gdp       | Log of government revenue from resource taxes and fees (% GDP)                             | UNU - WIDER GRD                            |
| ln_total_taxes_revenue        | Log of total government revenue from taxes                                                 | UNU - WIDER GRD                            |

#### Secrecy and tax

|                         |                                                                              |                                                           |
|-------------------------|------------------------------------------------------------------------------|-----------------------------------------------------------|
| Total FSI               | Financial Secrecy Score                                                      | TJN                                                       |
| cit                     | Statutory Corporate Income tax rates                                         | Mean 2014 - 2018, Janský, Petr; Palanský, Miroslav (2019) |
| cthi                    | Corporate Tax Haven Score                                                    | TJN                                                       |
| etr_real                | Effective tax rate, capped at 0.6 and using CIT for missing and non-reported | CBCR weighted average                                     |
| ln_cit                  | Log of cit                                                                   | KPMG, EY, PwC                                             |
| ln_etr_real             | Log of etr_real                                                              | CBCR weighted average                                     |
| tax_complex             | Time to prepare and pay taxes (hours)                                        | Mean 2014 - 2018, IC.TAX.DURS (WBD)                       |
| ln_accountant_d         | Log of number of accountants                                                 | LinkedIn (Garcia-Bernardo and Stausholm, Forthcoming)     |
| ln_all_tax              | Log of number of all tax professionals                                       | LinkedIn (Garcia-Bernardo and Stausholm, Forthcoming)     |
| ln_audience             | Log of number of linkedin users                                              | LinkedIn (Garcia-Bernardo and Stausholm, Forthcoming)     |
| ln_banker               | Log of number of bankers                                                     | LinkedIn (Garcia-Bernardo and Stausholm, Forthcoming)     |
| ln_ceo                  | Log of number of CEOs                                                        | LinkedIn (Garcia-Bernardo and Stausholm, Forthcoming)     |
| ln_cfo                  | Log of number of CFOs                                                        | LinkedIn (Garcia-Bernardo and Stausholm, Forthcoming)     |
| ln_coo                  | Log of number of COOs                                                        | LinkedIn (Garcia-Bernardo and Stausholm, Forthcoming)     |
| ln_cxo                  | Log of number of Chief Executives                                            | LinkedIn (Garcia-Bernardo and Stausholm, Forthcoming)     |
| ln_engineer             | Log of number of engineers in country                                        | LinkedIn (Garcia-Bernardo and Stausholm, Forthcoming)     |
| ln_finance              | Log of number of finance workers                                             | LinkedIn (Garcia-Bernardo and Stausholm, Forthcoming)     |
| ln_other_corporate      | Log of number of corporate tax professionals                                 | LinkedIn (Garcia-Bernardo and Stausholm, Forthcoming)     |
| ln_wealth               | Log of number of wealth managers                                             | LinkedIn (Garcia-Bernardo and Stausholm, Forthcoming)     |
| ln_transfer_pricing     | Log of number of transfer pricing specialists                                | LinkedIn (Garcia-Bernardo and Stausholm, Forthcoming)     |
| ln_tax_compliance_audit | Log of number of tax compliance experts and auditors                         | LinkedIn (Garcia-Bernardo and Stausholm, Forthcoming)     |
